# Supplementary material for: Entanglement-based dc magnetometry with separated ions
Source: arXiv:1704.01793 source file (2017-04-06)
Supplement: Supplementary file 1 [file supplemental_material12.pdf]

# Entanglement-based dc magnetometry with separated ions: supplemental material

T. Ruster,[1] H. Kaufmann,[1] M. A. Luda,[1,*] V. Kaushal,[1]
C. T. Schmiegelow,[1,†] F. Schmidt-Kaler,[1] and U. G. Poschinger[1]

[1]*Institut für Physik, Universität Mainz, Staudingerweg 7, 55128 Mainz, Germany*

## I. THE AC ZEEMAN EFFECT: HAMILTONIAN

In the following, we derive how an oscillating magnetic field affects the phase accumulation rate of magnetic sublevels of the $S_{1/2}$ and $D_{5/2}$ states. The linear Zeeman effect, caused by an homogenous magnetic field $\mathbf{B} = (0, 0, B)$, is described by the Hamiltonian

$$\hat{H}_0 = -\hat{\boldsymbol{\mu}}_{\text{eff}} \cdot \mathbf{B} = g\frac{e}{2m_e}\hat{\mathbf{J}} \cdot \mathbf{B} = g\frac{\mu_{\text{B}}}{\hbar}\hat{J}_z \cdot B \tag{1}$$

with $\mu_{\text{B}} = \frac{e\hbar}{2m_e}$. The energy eigenvalues are

$$E_m = g\mu_{\text{B}} m B = m\hbar\omega_{\text{L}} \tag{2}$$

with the Larmor frequency $\omega_{\text{L}} = g\mu_{\text{B}}\frac{B}{\hbar}$ and $m = -j, -j+1, \ldots, j$. The eigenstates are $|j, m\rangle$. For the $S_{1/2}$ state, the total angular momentum quantum number is $j = 1/2$, and for the $D_{5/2}$ state, it is $j = 5/2$.

We now add an interaction with an oscillating magnetic field $\mathbf{B}_{\text{rf}} = \left(B_{\text{rf},\perp}\cos(\Omega_{\text{rf}}t), 0, B_{\text{rf},\parallel}\cos(\Omega_{\text{rf}}t)\right)$ to the Hamiltonian:

$$\hat{H}(t) = \hat{H}_0 + V(t) \tag{3}$$

$$V(t) = 2\Omega_\perp \hat{J}_x\cos(\Omega_{\text{rf}}t) + 2\Omega_\parallel \hat{J}_z \cos(\Omega_{\text{rf}}t) \tag{4}$$

with $\Omega_\perp = \frac{1}{2}g\frac{\mu_{\text{B}}}{\hbar}B_{\text{rf},\perp}$ and $\Omega_\parallel = \frac{1}{2}g\frac{\mu_{\text{B}}}{\hbar}B_{\text{rf},\parallel}$. Due to the rotational symmetry of $\hat{H}_0$, it is not necessary to include a $y$-component in the oscillating magnetic field. We now switch to the interaction picture. The interaction Hamiltonian is transformed as

$$\hat{V}_I(t) = \text{e}^{\text{i}\hat{H}_0 t/\hbar} V \text{e}^{-\text{i}\hat{H}_0 t/\hbar} \tag{5}$$

$$= 2\Omega_\parallel \hat{J}_z\cos(\Omega_{\text{rf}}t) + \text{e}^{\text{i}\omega_{\text{L}}t\hat{J}_z/\hbar} 2\Omega_\perp \hat{J}_x \cos(\Omega_{\text{rf}}t)\text{e}^{-\text{i}\omega_{\text{L}}t\hat{J}_z/\hbar} \tag{6}$$

We express $\hat{V}_I(t)$ in terms of the ladder operators

$$\hat{J}_\pm = \hat{J}_x \pm \text{i}\hat{J}_y \tag{7}$$

and obtain

$$\hat{V}_I(t) = 2\Omega_\parallel \hat{J}_z\cos(\Omega_{\text{rf}}t) + \Omega_\perp\cos(\Omega_{\text{rf}}t)\text{e}^{\text{i}\omega_{\text{L}}t\hat{J}_z/\hbar}\left(\hat{J}_+ + \hat{J}_-\right)\text{e}^{-\text{i}\omega_{\text{L}}t\hat{J}_z/\hbar} \tag{8}$$

By writing down the matrix elements of $\hat{J}_z$ and $\hat{J}_\pm$ and performing the matrix multiplications, we find

$$\hat{V}_I(t) = 2\Omega_\parallel \hat{J}_z\cos(\Omega_{\text{rf}}t) + \Omega_\perp\cos(\Omega_{\text{rf}}t)\left(\hat{J}_+\text{e}^{\text{i}\omega_{\text{L}}t} + \hat{J}_-\text{e}^{-\text{i}\omega_{\text{L}}t}\right) \tag{9}$$

$$= 2\Omega_\parallel \hat{J}_z\cos(\Omega_{\text{rf}}t) + \frac{1}{2}\Omega_\perp\left(\hat{J}_+\left(\text{e}^{\text{i}(\omega_{\text{L}}+\Omega_{\text{rf}})t} + \text{e}^{\text{i}(\omega_{\text{L}}-\Omega_{\text{rf}})t}\right) + \hat{J}_-\left(\text{e}^{-\text{i}(\omega_{\text{L}}+\Omega_{\text{rf}})t} + \text{e}^{-\text{i}(\omega_{\text{L}}-\Omega_{\text{rf}})t}\right)\right) \tag{10}$$

In the following, we use the definitions $\delta = \omega_{\text{L}} - \Omega_{\text{rf}}$ and $\Sigma = \omega_{\text{L}} + \Omega_{\text{rf}}$. Then, the interaction Hamiltonian is

$$\hat{V}_I(t) = 2\Omega_\parallel \hat{J}_z\cos(\Omega_{\text{rf}}t) + \frac{\Omega_\perp}{2}\left(\hat{J}_+\left(\text{e}^{\text{i}\Sigma t} + \text{e}^{\text{i}\delta t}\right) + \hat{J}_-\left(\text{e}^{-\text{i}\Sigma t} + \text{e}^{-\text{i}\delta t}\right)\right) \tag{11}$$

---

* Present address: DEILAP, CITEDEF & CONICET, J.B. de La Salle 4397, 1603 Villa Martelli, Buenos Aires, Argentina

† Present address: Departamento de Física, FCEyN, UBA and IFIBA, Conicet, Pabellón 1, Ciudad Universitaria, 1428 Buenos Aires, Argentina

## II. THE AC ZEEMAN EFFECT: SOLUTION OF THE SCHRÖDINGER EQUATION

We solve the time-dependent Schrödinger equation in the interaction picture

$$\mathrm{i}\hbar \frac{\mathrm{d}}{\mathrm{d}t} |\Psi(t)\rangle_I = \hat{V}_I(t) |\Psi(t)\rangle_I \tag{12}$$

with a similar approach as presented in [1]. We write the interaction picture state as a general superposition of Zeeman sublevels of the electronic state:

$$|\Psi(t)\rangle_I = \sum_{m=-j}^{j} c_m(t) |j, m\rangle \tag{13}$$

Upon multiplying Eq. 12 with $\langle j, n|$, we obtain the set of equations

$$\mathrm{i}\hbar\, \dot{c}_n(t) = \sum_{m=-j}^{j} c_m(t) \langle j, n| \hat{V}_I(t) |j, m\rangle \tag{14}$$

where $n = -j, -j+1, \ldots, j$. As we are only interested in dispersive effects, we assume that the populations $|c_n(t)|$ do not change over time. Then, it is beneficial to write

$$c_n(t) \approx c_n(0)\, \mathrm{e}^{-\mathrm{i}\varphi_n(t)} \tag{15}$$

The time derivative is

$$\dot{c}_n(t) = -\mathrm{i}\, c_n(0)\, \dot{\varphi}_n(t)\, \mathrm{e}^{-\mathrm{i}\varphi_n(t)} \tag{16}$$

In the first step, we assume that the accumulated phase is small, i.e. $\mathrm{e}^{-\mathrm{i}\varphi_n(t)} \approx 1$. Then, the phase accumulation rate is given by

$$\dot{\varphi}_n(t) \approx \frac{\mathrm{i}}{c_n(0)} \dot{c}_n(t) = \frac{1}{\hbar c_n(0)} \sum_{m=-j}^{j} \langle j, n| \hat{V}_I(t) |j, m\rangle\, c_m(t) \tag{17}$$

where we inserted Eq. 14 in the last step. Additionally, we cast Eq. 14 into an integral equation

$$\mathrm{i}\hbar\, c_n(t) = \sum_{m=-j}^{j} \int_0^t c_m(t) \langle j, n| \hat{V}_I(t') |j, m\rangle\, \mathrm{d}t' \;\approx\; \sum_{m=-j}^{j} c_m(0) \langle j, n| \int_0^t \hat{V}_I(t')\mathrm{d}t' \,|j, m\rangle \tag{18}$$

We insert the integral equation into Eq. 17 and obtain

$$\begin{aligned} \dot{\varphi}_n(t) &\approx \frac{1}{\mathrm{i}\hbar^2 c_n(0)} \sum_{m=-j}^{j} \sum_{k=-j}^{j} c_k(0) \langle j, n| \hat{V}_I(t) |j, m\rangle \langle j, m| \int_0^t \hat{V}_I(t')\mathrm{d}t' \,|j, k\rangle \\ &= \frac{1}{\mathrm{i}\hbar^2 c_n(0)} \sum_{k=-j}^{j} c_k(0) \langle j, n| \hat{V}_I(t) \int_0^t \hat{V}_I(t')\mathrm{d}t' \,|j, k\rangle \end{aligned} \tag{19}$$

Then, we consider the product

$$\begin{aligned} V_I(t) \int_0^t \hat{V}_I(t')\mathrm{d}t' = &\left(2\Omega_\parallel \hat{J}_z \cos(\Omega_{\mathrm{rf}} t) + \frac{\Omega_\perp}{2} \hat{J}_+ \left(\mathrm{e}^{\mathrm{i}\Sigma t} + \mathrm{e}^{\mathrm{i}\delta t}\right) + \frac{\Omega_\perp}{2} \hat{J}_- \left(\mathrm{e}^{-\mathrm{i}\Sigma t} + \mathrm{e}^{-\mathrm{i}\delta t}\right)\right) \quad \times \\ \times \quad &\left(\frac{2\Omega_\parallel}{\Omega_{\mathrm{rf}}} \hat{J}_z \sin(\Omega_{\mathrm{rf}} t) + \frac{\Omega_\perp}{2} \hat{J}_+ \left(\frac{\mathrm{e}^{\mathrm{i}\Sigma t} - 1}{\mathrm{i}\Sigma} + \frac{\mathrm{e}^{\mathrm{i}\delta t} - 1}{\mathrm{i}\delta}\right) + \frac{\Omega_\perp}{2} \hat{J}_- \left(\frac{\mathrm{e}^{-\mathrm{i}\Sigma t} - 1}{-\mathrm{i}\Sigma} + \frac{\mathrm{e}^{-\mathrm{i}\delta t} - 1}{-\mathrm{i}\delta}\right)\right) \end{aligned} \tag{20}$$

After time averaging, the only relevant terms are

$$V_I(t) \int_0^t \hat{V}_I(t')\mathrm{d}t' = -\mathrm{i} \frac{\Omega_\perp^2}{4} \left(\hat{J}_- \hat{J}_+ - \hat{J}_+ \hat{J}_-\right) \left(\frac{1}{\Sigma} + \frac{1}{\delta}\right) \tag{21}$$

Due to the commutator relation $\left[\hat{J}_+, \hat{J}_-\right] = 2\hbar\hat{J}_z$, this simplifies to

$$V_I(t)\int_0^t \hat{V}_I(t')\mathrm{d}t' = \mathrm{i}\hbar\frac{\Omega_\perp^2}{2}\hat{J}_z\left(\frac{1}{\Sigma}+\frac{1}{\delta}\right) \tag{22}$$

Plugging this into Eq. 19, the sum collapses and we obtain the time-averaged phase accumulation rate

$$\overline{\dot{\varphi}_n} = \frac{\Omega_\perp^2}{2}n\left(\frac{1}{\Sigma}+\frac{1}{\delta}\right) = n\Omega_\perp^2\frac{\omega_\mathrm{L}}{\omega_\mathrm{L}^2-\Omega_\mathrm{rf}^2} \tag{23}$$

for each Zeeman sublevel $n$. We describe the ac Zeeman shift by the differential phase accumulation rate of the populated sublevels $m_1$ and $m_2$

$$\omega^{(\mathrm{ac},1)} := \overline{\dot{\varphi}_{m_1}} - \overline{\dot{\varphi}_{m_2}} = \Delta m\left(g\frac{\mu_\mathrm{B}}{2\hbar}B_{\mathrm{rf},\perp}\right)^2\frac{\omega_\mathrm{L}}{\omega_\mathrm{L}^2-\Omega_\mathrm{rf}^2} \tag{24}$$

with $\Delta m = m_1 - m_2$. Since the phase is linearly accumulating with time, the assumption $\mathrm{e}^{-\mathrm{i}\varphi_n(t)} \approx 1$ does not hold for large evolution times. To obtain a more accurate result, we solve the differential equation 14 again, but with the revised assumption $\mathrm{e}^{-\mathrm{i}\varphi_n(t)} = \mathrm{e}^{-\mathrm{i}\omega^{(\mathrm{ac})}t}$. This leads to a similar expression:

$$\omega^{(\mathrm{ac})} = \Delta m\left(g\frac{\mu_\mathrm{B}}{2\hbar}B_{\mathrm{rf},\perp}\right)^2\frac{\nu}{\nu^2-\Omega_\mathrm{rf}^2}, \tag{25}$$

where the Larmor frequency $\omega_\mathrm{L}$ is replaced by the total absolute frequency splitting between neighboring magnetic sublevels

$$\nu := \hbar\omega_\mathrm{L} + \hbar\omega^{(\mathrm{ac})}. \tag{26}$$

Note that this quantity is experimentally accessible.

## III. SEPARATION OF DC AND AC MAGNETIC FIELDS

In the experiment, we find that both dc and ac Zeeman shifts are position-dependent. We measure *differences* of atomic frequency splittings between two locations $x_1$ and $x_2$ along the trap axis of a linear segmented ion trap. In order to distinguish the dc and ac Zeeman frequency shifts, we measure the differential phase accumulation rates in the $\mathrm{S}_{1/2}$ ground state with $\Delta m = 1$, and in the $\mathrm{D}_{5/2}$ metastable state with $\Delta m = 5$, given by

$$\Delta\omega_\mathrm{S}(x_1,x_2) = \frac{g_\mathrm{S}\mu_\mathrm{B}}{\hbar}\Delta B(x_1,x_2) + \Delta\omega_\mathrm{S}^{(\mathrm{ac})}(x_1,x_2) \tag{27}$$

$$\Delta\omega_\mathrm{D}(x_1,x_2) = \frac{5g_\mathrm{D}\mu_\mathrm{B}}{\hbar}\Delta B(x_1,x_2) + \Delta\omega_\mathrm{D}^{(\mathrm{ac})}(x_1,x_2) \tag{28}$$

with $\Delta B(x_1,x_2) = B(x_1) - B(x_2)$ and $\Delta\omega_J^{(\mathrm{ac})}(x_1,x_2) = \omega_J^{(\mathrm{ac})}(x_1) - \omega_J^{(\mathrm{ac})}(x_2)$. Here, $J$ denotes the electronic state ($J \equiv \mathrm{S}$ for the $\mathrm{S}_{1/2}$ state, and $J \equiv \mathrm{D}$ for the $\mathrm{D}_{5/2}$ state). To obtain the static magnetic field difference, we write Eq. 28 as

$$\Delta\omega_\mathrm{D}(x_1,x_2) = \frac{5g_\mathrm{D}\mu_\mathrm{B}}{\hbar}\Delta B(x_1,x_2) + \chi\Delta\omega_\mathrm{S}^{(\mathrm{ac})}(x_1,x_2) \tag{29}$$

with the ac Zeeman difference ratio

$$\chi \equiv \Delta\omega_\mathrm{D}^{(\mathrm{ac})}(x_1,x_2)/\Delta\omega_\mathrm{S}^{(\mathrm{ac})}(x_1,x_2). \tag{30}$$

We insert Eq. 27 into Eq. 29 and solve for the static magnetic field difference

$$\Delta B(x_1,x_2) = \frac{\hbar}{\mu_\mathrm{B}}\frac{\Delta\omega_\mathrm{D}(x_1,x_2) - \chi\Delta\omega_\mathrm{S}(x_1,x_2)}{5g_\mathrm{D} - \chi g_\mathrm{S}}. \tag{31}$$

To extract $\Delta\omega_J^{(\mathrm{ac})}(x_1,x_2)$ from measurements, we insert Eq. 31 into Eq. 27 or 28 and obtain

$$\Delta\omega_J^{(\mathrm{ac})}(x_1,x_2) = \Delta\omega_J(x_1,x_2) - \Delta m\, g_J\frac{\Delta\omega_\mathrm{D}(x_1,x_2) - \chi\Delta\omega_\mathrm{S}(x_1,x_2)}{5g_\mathrm{D} - \chi g_\mathrm{S}}. \tag{32}$$

The ac Zeeman difference ratio is given by

$$\chi(x_1,x_2)=\frac{\Delta\omega_{\mathrm{D}}^{(\mathrm{ac})}(x_1,x_2)}{\Delta\omega_{\mathrm{S}}^{(\mathrm{ac})}(x_1,x_2)}=5\left(\frac{g_{\mathrm{D}}}{g_{\mathrm{S}}}\right)^2\frac{B_{\mathrm{rf},\perp}(x_1)^2\frac{\nu_{\mathrm{D}}(x_1)}{\nu_{\mathrm{D}}(x_1)^2-\Omega_{\mathrm{rf}}^2}-B_{\mathrm{rf},\perp}(x_2)^2\frac{\nu_{\mathrm{D}}(x_2)}{\nu_{\mathrm{D}}(x_2)^2-\Omega_{\mathrm{rf}}^2}}{B_{\mathrm{rf},\perp}(x_1)^2\frac{\nu_{\mathrm{S}}(x_1)}{\nu_{\mathrm{S}}(x_1)^2-\Omega_{\mathrm{rf}}^2}-B_{\mathrm{rf},\perp}(x_2)^2\frac{\nu_{\mathrm{S}}(x_2)}{\nu_{\mathrm{S}}(x_2)^2-\Omega_{\mathrm{rf}}^2}}. \tag{33}$$

Here, both the total absolute frequency splittings $\nu_J(x)$ and oscillating magnetic fields $B_{\mathrm{rf},\perp}(x)^2$ are position-dependent. As an approximation, we discard the position-dependence:

$$\nu_J(x)\approx\nu_J(x_{\mathrm{LIZ}}), \tag{34}$$

where $\nu_J(x_{\mathrm{LIZ}})$ denotes the *absolute* frequency splitting at the laser interaction zone (LIZ). Now, Eq. 33 simplifies to

$$\chi\approx 5\left(\frac{g_{\mathrm{D}}}{g_{\mathrm{S}}}\right)^2\frac{\nu_{\mathrm{D}}(x_{\mathrm{LIZ}})}{\nu_{\mathrm{S}}(x_{\mathrm{LIZ}})}\cdot\frac{\nu_{\mathrm{S}}(x_{\mathrm{LIZ}})^2-\Omega_{\mathrm{rf}}^2}{\nu_{\mathrm{D}}(x_{\mathrm{LIZ}})^2-\Omega_{\mathrm{rf}}^2}. \tag{35}$$

With values for $\nu_{\mathrm{S,D}}(x_{\mathrm{LIZ}})$ available, we can determine a value for $\chi$, which can be inserted into Eqs. 31,32 to obtain the desired quantities.

## IV. ERROR CHARACTERIZATION

To compute a value for $\chi$ according to Eq. 35, the required values for the total frequency splittings at the laser interaction zone $\nu_{\mathrm{S,D}}(x_{\mathrm{LIZ}})$ are obtained from direct laser spectroscopy on a single ion. For $J=\mathrm{S}$, spectroscopy is carried out on the stimulated Raman transition, while for $J=\mathrm{D}$, the $\mathrm{S}_{1/2}\leftrightarrow\mathrm{D}_{5/2}$ quadrupole transition is utilized. In both cases, an interrogation time of 200 $\mu$s yields an accuracy of better than $2\pi\cdot 1$ kHz, such that we obtain $\nu_{\mathrm{S}}(x_{\mathrm{LIZ}})=2\pi\cdot 10.2136(10)$ MHz, $\nu_{\mathrm{D}}(x_{\mathrm{LIZ}})=2\pi\cdot 6.1231(6)$ MHz, and therefore $\chi=1.00946(16)$. Since the absolute frequency splittings exceed their inhomogeneities along the trap axis by more than 3 orders of magnitude, it is justified to discard the position-dependence in Eq. 34.

The relative accuracy of the magnetic field difference is reduced with respect to the bare measurements of differential phase accumulation rates, as $\Delta B$ according to Eq. 31 is affected by statistical uncertainties of $\Delta\omega_{\mathrm{S}},\Delta\omega_{\mathrm{D}}$ and $\chi$. Gaussian error propagation yields relative uncertainties which are increased by a factor of about 2 as compared to the differential frequency measurements.

In the following, we further analyze the validity of the approximation Eq. 34. To this end, we compare the ac Zeeman ratio from the approximation Eq. 35 to a self-consistent estimate from the exact expression Eq. 33. For the latter, we obtain the local frequency splittings $\nu_J(x)$ via

$$\nu_J(x)=\Delta\omega_J(x,x_{\mathrm{LIZ}})/\Delta m_J+\nu_J(x_{\mathrm{LIZ}}) \tag{36}$$

In order to obtain estimates for $B_{\mathrm{rf},\perp}(x)^2$, we first compute the absolute ac Zeeman splittings at the laser interaction zone $\omega_J^{(\mathrm{ac})}(x_{\mathrm{LIZ}})$ from the single-ion version of Eq. 32:

$$\omega_J^{(\mathrm{ac})}(x_{\mathrm{LIZ}})=\omega_J(x_{\mathrm{LIZ}})-\Delta m\, g_J\frac{\omega_{\mathrm{D}}(x_{\mathrm{LIZ}})-\chi\omega_{\mathrm{S}}(x_{\mathrm{LIZ}})}{5g_{\mathrm{D}}-\chi g_{\mathrm{S}}}. \tag{37}$$

Here, we employ $\chi$ from expression Eq. 35, which is *exact* for the single-ion case. Now, using

$$\omega_J^{(ac)}(x)=\Delta\omega_J^{(\mathrm{ac})}(x,x_{\mathrm{LIZ}})+\omega_J^{(\mathrm{ac})}(x_{\mathrm{LIZ}}), \tag{38}$$

we obtain the inhomogeneous ac magnetic field according to Eq. 25:

$$B_{\mathrm{rf},\perp}(x)^2=\frac{\omega_J^{(\mathrm{ac})}(x)}{\Delta m}\left(\frac{2\hbar}{g\mu_{\mathrm{B}}}\right)^2\frac{\nu_J(x)^2-\Omega_{\mathrm{rf}}^2}{\nu_J(x)}. \tag{39}$$

Inserting the results from Eqs. 36,39 into Eq. 33, we obtain position dependent values for $\chi(x_1,x_2)$. Comparing resulting values of $\Delta B(x_1,x_2)$ and $\Delta\omega_J^{(\mathrm{ac})}(x_1,x_2)$, we find deviations of less than 1% of the statistical uncertainty across the entire region of interest. We therefore conclude that Eq. 35 is an excellent approximation.

---

[1] D. Budker, D. F. Kimball, and D. P. DeMille, *Atomic physics : an exploration through problems and solutions*, second edition ed. (Oxford University Press, Oxford, 2008) pp. 98–100.
